# Supplementary material for: Mapping Image Potential States on Graphene Quantum Dots
Source: arXiv:1303.1800 source file (2013-06-14)
Supplement: Supplementary file 1 [file supplementary.pdf]

# Mapping Image Potential States on Graphene Quantum Dots
# Supplementary Information

Fabian Craes,[1,*] Sven Runte,[1] Jürgen Klinkhammer,[1] Marko Kralj,[2] Thomas Michely,[1] and Carsten Busse[1]

[1] *II. Physikalisches Institut, Universität zu Köln, Zülpicher Straße 77, 50937 Köln, Germany*

[2] *Institut za fiziku, Bijenička 46, 10000 Zagreb, Croatia*

(Dated: June 13, 2013)

## INFLUENCE OF STARK SHIFT

Here, we will address the influence of the Stark shift on our experiment. The electric field causing this shift depends in a complex way on the distance $z$ from the surface (unless a very large tip radius is assumed), governed by the bias voltage $U$ and the distance $z_0$ between the tip and the sample. As these quantities are slightly different for the same image potential state (IPS) measured on different graphene quantum dots (GQDs), one could speculate that these states are Stark-shifted in a different way, making a quantitative analysis impossible. We asses the contribution of the Stark effect by performing $I_{\mathrm{stab}}$- and thus $z_0$-dependent measurements of $E^{(2)}$ on pristine Ir(111). We approximate the field by assuming a simple capacitor model with $F = U/z_0$ [1]. Increasing $I_{\mathrm{stab}}$ from 0.2 nA to 0.3 nA changes the field by $\Delta F = 0.87\,\mathrm{V/nm}$. At the same time $E^{(2)}$ changes by $\Delta E \simeq 40\,\mathrm{mV}$. In the size-dependent measurements on GNFs, the field changes by almost the same value $\Delta F = 0.90\,\mathrm{V/nm}$ for the measurements of $E^{(2)}$ between the smallest and the largest flakes under the assumption of $z_0 = 0.5\,\mathrm{nm}$ for $I_{\mathrm{stab}} = 0.2$ nA. The observed shift in the energy of this state between two states, however, is $\Delta E \simeq 670\,\mathrm{mV}$ and thus more than an order of magnitude larger as the Stark shift measured above, proving that the energy shift is indeed dominated by confinement effects. Another influence of the electric field of the tip in general is the non-conservation of $k_{||}$ [2]. In our case confinement on small nanostructures allows only well defined discrete values. But the effect definately influences the measured local density of states (LDOS) at the qunatum dot boundary region, which we do not adress in this work.

## IPS-2DEG INTERACTION

Fig. 1 shows a matrix plot of the $\mathrm{d}I/\mathrm{d}U(E - E_F)$ data of a series of 80 point spectra measured on a line across a perfectly hexagonal GQD [inset of Fig. 1]. $E^{(n)}$ is decreased on the flake with respect to Ir(111) due to the lowered $\Phi$. For the boundary region itself, note that the first state shows an abrupt, all higher orders a more continuous way of change. Regarding this observation, both a spill-out of the confined gr-IPSs and a penetration of Ir-IPSs into the area over the flake should be considered [3]. On this view Fig. 1 indicates a suppressed interaction for $n = 1$ and interacting two dimensional electron gases (IPS-2DEGs) of the flake and the surrounding substrate for $n > 1$. The pronounced fine structure of $n = 1$ is again due to the shift through the dominant states $(m, l)$ with energy. It can be inferred from Fig. 2 (b) (main text) that for small flakes the energy region of visible confinement states extends up to the next IPS. The complex structure found for high $n$ is probably due to an interpenetration of Ir and graphene IPSs or results from a change in the most dominating state for high values of $U$ and $z_0$ or a combination of both.

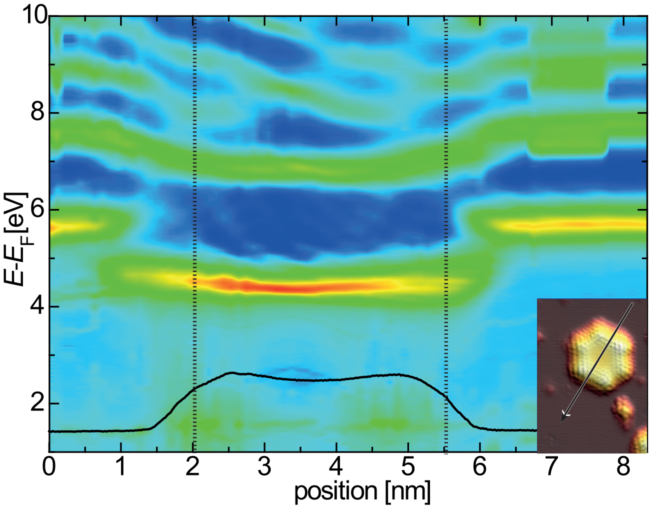


FIG. 1. (color online). Matrix plot of $\mathrm{d}I/\mathrm{d}U$ point spectra across an $\Omega = 13\,\mathrm{nm}^2$ GQD (color scale from blue to red), $U_{\mathrm{stab}} = 0.7\,\mathrm{V}$, $I_{\mathrm{stab}} = 0.2\,\mathrm{nA}$, dashed vertical lines indicating border of the flake; thin black line is a line profile through the topography of the island as indicated in the inset; inset: topography, size $6.8 \times 9.4\,\mathrm{nm}^2$, $U = 712\,\mathrm{mV}$, $I = 0.4\,\mathrm{nA}$.

## EXTENDED GRAPHENE

We state that the largest GQDs resemble extended epitaxial graphene. Especially the biggest GQD with an area of 378 $\mathrm{nm}^2$ at hand in this work shows a $\mathrm{d}I/\mathrm{d}U$ spectrum without any signature of confinement substructure (see Fig. 2).

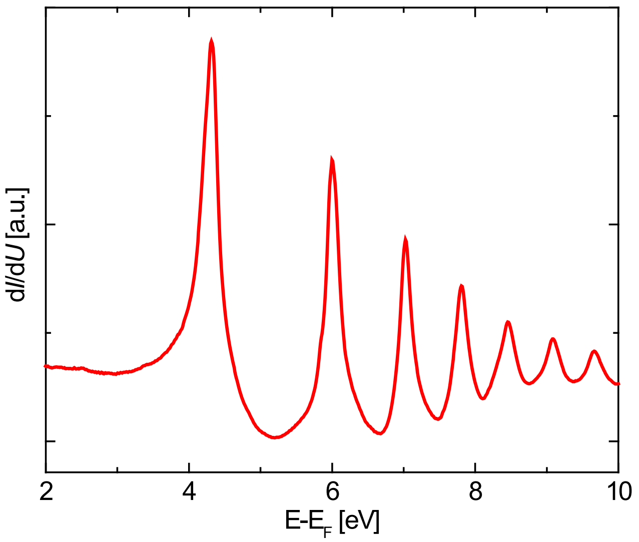


FIG. 2. (color online). d$I$/d$U$ point spectrum on the $\Omega = 378\,\mathrm{nm}^2$ GQD (G) in Fig. 1 (b) (main text), $U_{\mathrm{stab}} = 1\,\mathrm{V}$, $I_{\mathrm{stab}} = 0.2\,\mathrm{nA}$.

* craes@ph2.uni-koeln.de

[1] P. Wahl, M. A. Schneider, L. Diekhöner, R. Vogelgesang, and K. Kern, Phys. Rev. Lett. **91**, 106802 (2003).
[2] J. I. Pascual, C. Corriol, G. Ceballos, I. Aldazabal, H.-P. Rust, K. Horn, J. M. Pitarke, P. M. Echenique, and A. Arnau, Phys. Rev. B **75**, 165326 (2007).
[3] K. Schouteden and C. Van Haesendonck, Phys. Rev. Lett. **103**, 266805 (2009).
